# Supplementary material for: An Adaptive Intelligence Algorithm for Undersampled Knee MRI Reconstruction
Source: arXiv:2004.07339 source file (2020-10-27)
Supplement: Supplementary file 1 [file supplementary.tex]

\begin{table*}[!tb]

\centering
\caption{\label{table:supp_img}top to bottom: Ground truth, Zero-filled}
\resizebox{1.\width}{!}{\input{supplementary/image}}
\end{table*}

\begin{table*}[!tb]

\centering
\caption{\label{table:supp_singel_step_loss}Qualitative results for single loss function, top to bottom: Huber, SSIM, SSIM\_challenge, MSSIM, 0.84MSSIM+0.16L1}
\resizebox{1.\width}{!}{\input{supplementary/singel_step_loss}}
\end{table*}

\begin{table*}[!tb]

\centering
\caption{\label{table:supp_two_step_loss}Qualitative results for two step training, top to bottom: (10$\&$15) L1$\&$SSIM, MSE$\&$L1, MSE$\&$SSIM,SSIM$\&$MSE,SSIM$\&$L1}
\resizebox{1.\width}{!}{\input{supplementary/two_step_loss}}
\end{table*}

\begin{table*}[!tb]

\centering
\caption{\label{table:supp_supp_opt}Qualitative results for optimizers, top to bottom: Radam, Look Ahead, Ranger}
\resizebox{1.\width}{!}{\input{supplementary/optimizers}}
\end{table*}

\begin{table*}[!tb]

\centering
\caption{\label{table:supp_struct}Qualitative results for GANs, top to bottom: GAN, WGAN}
\resizebox{1.\width}{!}{\input{supplementary/structures}}
\end{table*}

\begin{table*}[!tb]

\centering
\caption{\label{table:supp_attention}Qualitative results for attention gate}
\resizebox{1.\width}{!}{\input{supplementary/attention}}
\end{table*}
